# Supplementary material for: Iterative Refinement for Real-Time Multi-Robot Path Planning
Source: arXiv:2102.12331 source file (2021-07-26)
Supplement: Supplementary file 1 [file appendix.tex]

\section*{Appendix*}
